# Supplementary material for: Semantically-Aware Strategies for Stereo-Visual Robotic Obstacle Avoidance
Source: arXiv:2107.06401 source file (2021-07-13)
Supplement: Supplementary file 1 [file 6_appendix.tex]

\section*{APPENDIX}
